# Supplementary material for: Graph-based Cluttered Scene Generation and Interactive Exploration using Deep Reinforcement Learning
Source: arXiv:2109.10460 source file (2021-09-21)
Supplement: Supplementary file 1 [file appendix.tex]

\subsection{Architecture}
Scene graphs form the backbone of our approach. Hence, to build our agents we use Message Passing Neural Networks (MPNNs) that can extract high level features from graphs by propagating messages between nodes. 
In what follows, we discuss the scene graph representations that we use as input, and the model architecture of our agents as well as the object detector. %below:

\textbf{Scene Generation Agent:} For the scene generation agent we represent the nodes of the scene graph as the concatenation of a one-hot vector encoding the node type, a boolean flag \textit{is\_simulated} that represents if the node has been simulated, and the $3$ dimensional position of the node if \textit{is\_simulated} is set to be True. The edges of the scene graph are represented as one-hot vectors that specify the type of the edge. Before feeding the scene graphs into a network, we first embed each node using a fully connected (FC) layer followed by a non-linearity (Leaky-ReLU), resulting in a vector of  $32$ dimensions. We use a similar network to embed the edges into a vector of size $3$. 
The network architecture is similar to the one used by \cite{janisch2020symbolic} for BlockWorld. 
Consider an input scene graph G consisting of nodes from $\mathcal{V}$ and edges from $\mathcal{E}$. A Message Passing Neural Network is defined by a message aggregating function $\phi_{agg}$ that aggregates incoming messages from all the neighbours of a node, an update function $\phi_{update}$ that updates the features of a given node based on the received messages and a message embedding function $\phi_{msg}$ that creates a message from a sender node $e.s$ to a receiver node $e.r$ over an edge $e$. In our experiments, we aggregate messages as follows: 
\begin{equation}
\forall v: m_{v}=\max _{e . r=v} \phi_{m s g}(e, e . s)
\label{eq:aggr_function}
\end{equation}
The aggregated messages are then used to update the node features:
\begin{equation}
\forall v: v^{\prime}=v+\phi_{a g g}\left(v, m_{v}, g\right)
\label{eq:update_function}
\end{equation}
Here $g$ represents a global node that embodies features from the entire graph using a Global Attention~\cite{li2015gated} Layer and a skip connection, defined as follows:
\begin{equation}
\left.g^{\prime}=g+\phi_{g l b}\left(g, \sum_{v \in \mathcal{V}} \phi_{a t t}(v) \cdot \phi_{\text {feat }}(v)\right)\right)
\label{eq:global_node}
\end{equation}
$\phi_{att}$ is a single liner layer followed by a softmax and $\phi_{feat}$ and $\phi_{glb}$ are single linear layers followed by a Leaky-ReLU. The above steps, equations \ref{eq:aggr_function}, \ref{eq:update_function}, \ref{eq:global_node}, denote one step of our Multi-Message Passing architecture. In our experiments, we repeat this step $4$ times and pass $g^{\prime}$ from the last step through a linear layer to generate the Q-values for all the rules in our graph grammar. See table \ref{tab:hyperparameters_scene_generation}, for details about hyper parameters.
% \deleted{ We train this agent with Soft Q-Learning for a total of $64k$ steps starting with a learning rate of $5\times 10^{-5}$ and halving it every $2k$ steps. The network architecture is similar to} \cite{janisch2020symbolic} \deleted{albeit we utilize $4$ message passing layers. We pass the output of the GlobalAttention layer through a FC layer to generate Q-values for all the rules in our graph grammar. We train the agent for a total of $64k$ steps starting with a learning rate of $5\times 10^{-5}$ and halving it every $2k$ steps.}
% Our network consists of $4$ message passing layers each of which has an FC layer that appends the node and edge features to create $32$ dimensional vector. We also use a Global Attention layer that consolidates from all nodes of the graph at each stage and passes it to the next stage. The aggregating function of each layer concatenates the node features with the global attention output and 

\textbf{Scene Exploration Agent:} It uses a similar scene graph representation with a few modifications. For the Privileged Agent, it uses an \textit{is\_seen} flag instead of an \textit{is\_simulated} flag to indicate whether an object has been seen or not. The node features also contain the orientation of the object represented as quaternions. The edges of this graph are represented with a single boolean flag to denote if the two objects are connected. 

    We use architecture identical to \cite{janisch2020symbolic} to compute the value of the state and actions. 
The privileged Scene Exploration agent computes the value of a state and a probability distribution over pick and place nodes as output. The value is computed by passing $g^{\prime}$ from the final Global Attention layer through a linear layer that outputs a single value for a given input state. To compute the probability distribution over nodes, the node features are passed through a linear layer that outputs a single value, which is then mapped to a probability distribution using a softmax function.
The same architecture is utilized for the Student Agent, but we drop the FC network that computes the value function as we directly maximize the log probabilities of the actions through Behavior Cloning from expert trajectories generated by the privileged Exploration Agent.

\textbf{Object detector:} We utilize the Scaled-YOLOv4 \cite{wang2020scaled} network as the object detector. First, we create simulated scenes by dropping $20$ objects (randomly sampled from the set of objects defined previously) into a bin and collect a dataset of 100k images. We then augment this dataset with 10k images of scenes generated by a random scene generation agent. In each case, we capture an image from the overhead RGBD camera and record the bounding box annotations for all objects in the scene. This data collection pipeline ensures that we include a significant proportion of partially and completely occluded objects in our dataset. We train the network on this dataset and use it as the object detector throughout our paper.
% \vspace{-50pt}
\hypscenegen

% Please add the following required packages to your document preamble:
% \usepackage{longtable}
% Note: It may be necessary to compile the document several times to get a multi-page table to line up properly
% \begin{longtable}[t]{|l|r|}
% \hline
% Hyperparameter & \multicolumn{1}{l|}{Value} \\ \hline
% \endfirsthead
% %
% \endhead
% %
% \hline
% \endfoot
% %
% \endlastfoot
% %
% Learning Rate & 1e-3 \\
% Discount Factor $\gamma$ & 0.99 \\
% Batch size & 64 \\
% Stability penalty $r_s$ & -0.2 \\
% Q range & \multicolumn{1}{l|}{(-15,15)} \\
% Target update factor $\rho$ & 0.005 \\
% Detection reward $r_d$ & 1.0 \\ \hline
% \caption{\added{Hyperparameters used for training the Scene Exploration Agent using A2C.}}
% \label{tab:hyperparameters_scene_exploration}\\
% \end{longtable}
\hypsceneexp
\subsection{Scene Grammar}
\scenegrammartable
\begin{figure*}[h]
\centering
\includegraphics[width=0.95\linewidth]{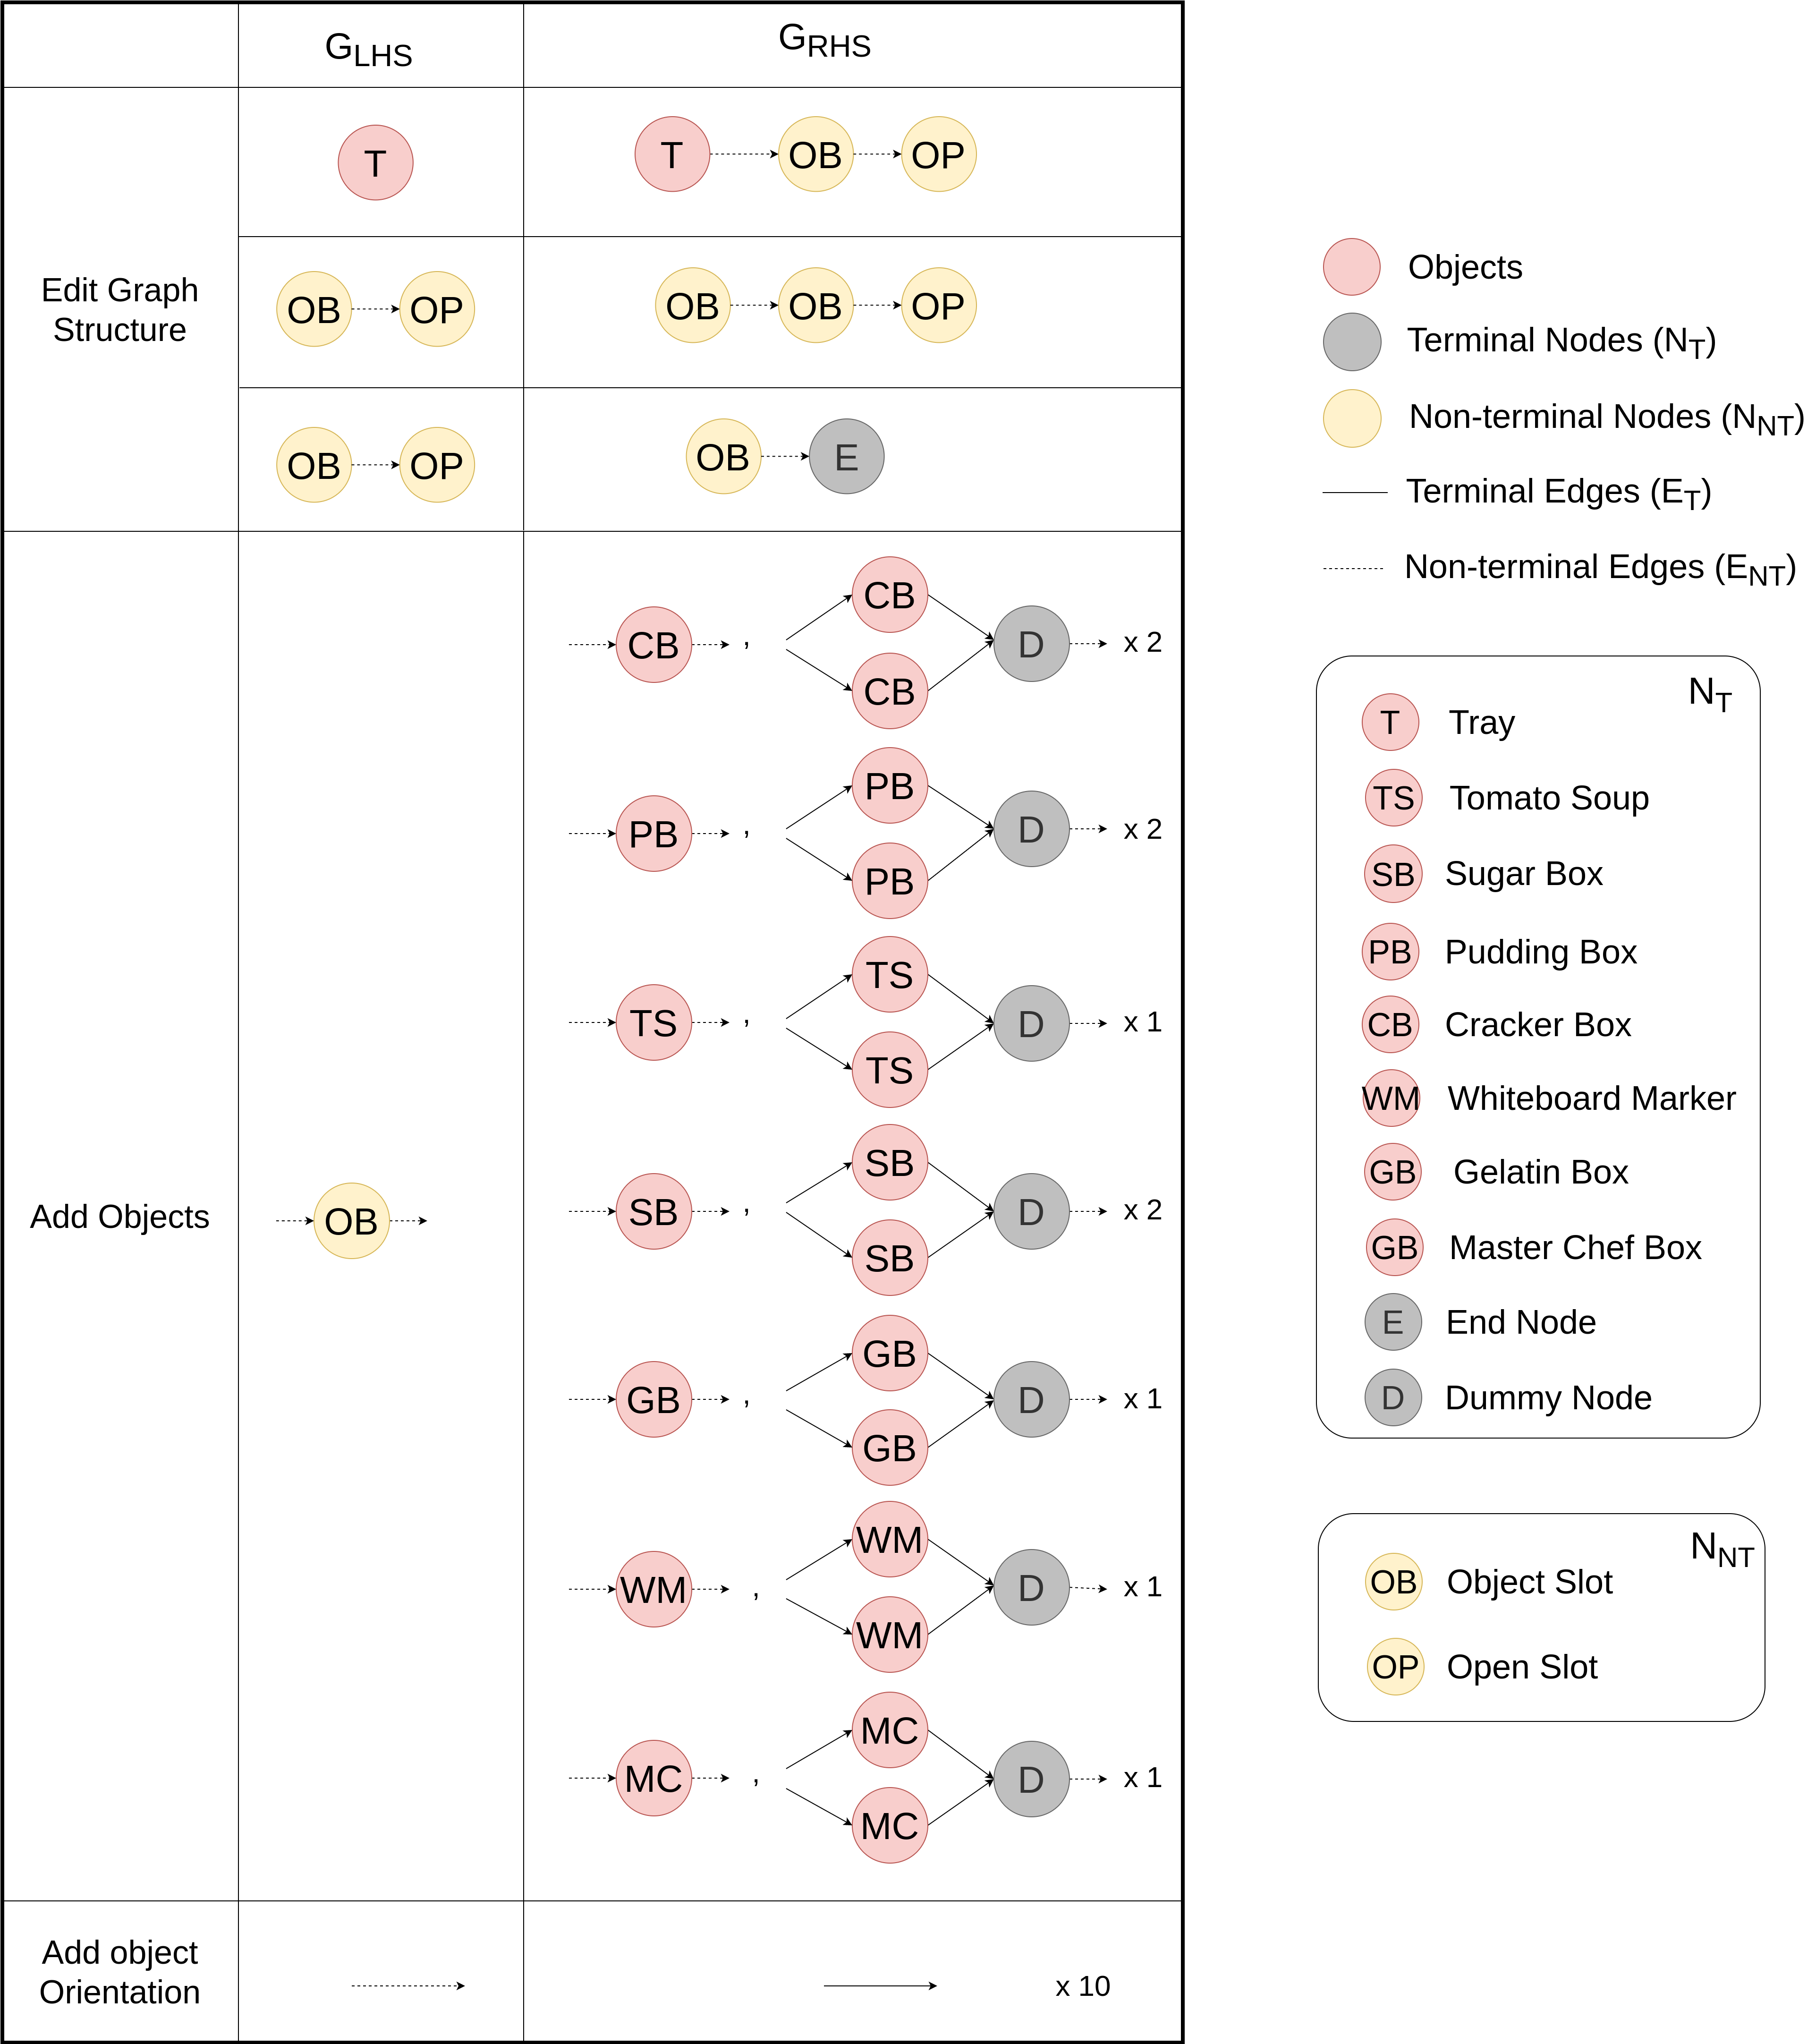}

\caption{The set of production rules available to the agent. When a rule is applied a subgraph $G_{LHS}$ is found in the input graph and is replaced by the subgraph $G_{RHS}$.}
% \sehoon{This is good. Can you add captions to the graph (with circles). People will not know it without reading figures.}}
\label{fig:all_production_rules}
\end{figure*}
Our scene grammar is defined by a set of production rules and a collection of terminal and non-terminal nodes. We list all the terminal and non-terminal nodes and their description in Table \ref{tab:scene_grammar_nodes}. Given these nodes, we can sequentially apply a set of production rules that evolve the scene graph by adding, removing or replacing subgraphs. In our work we use three types of production rules: 
\begin{enumerate}
    \item \textbf{Rules to edit the graph structure:} We define two rules, \textit{stack\_object} and \textit{drop\_object}, that add an \textit{object\_node} by stacking it on top of another existing object or dropping it on the tray, respectively. We also define an additional rule that replaces an \textit{open\_slot} with an \textit{end} node.
    \item \textbf{Rules to add objects:} We define $7$ rules that can substitute \textit{object\_node} with one of the $7$ objects available to the agent. We add $9$ additional \textit{meta\_object} rules that insert multiple object nodes all sharing a common parent. We use these rules to add multiple objects in close proximity to each other and allow stacking objects such that all the objects in the \textit{meta\_object} support the weight.
    \item \textbf{Rules to add object orientation:} We define $10$ rules, each corresponding to an orientation a chosen object can be placed in. Each of these rules takes any two nodes connected with a \textit{primitive} and replaces the edge with an orientation edge that represents the orientation of the child object in the scene.
\end{enumerate}
See Figure \ref{fig:all_production_rules} for the definition of all the production rules we use in our experiment. The multiplicative factor denotes the number of different configurations available for a particular rule. In total, we have $30$ production rules in our scene grammar.

\subsection{Simulation Details}
We use iGibson ~\cite{shen2020igibson} to simulate our scene generation and scene exploration pipeline. We specifically chose iGibson because it can utilize the GPU, allowing for high frame rate rendering. 

Every episode of the scene generation environment starts with an empty tray. At every step, the agent can choose a production rule and apply it on the corresponding scene graph to gradually grow it. 
Every time the scene graph reaches a state where all nodes are terminal, we realize the graph in the simulator, by building the corresponding scene. 
This scene is then rendered and used to compute the reward the agent should get. 
To compute the reward we pass the rendered image of the scene to an object detector and compare the output to the ground truth object bounding boxes. 
The reward the agent gets is proportional to the difference between the ground truth and predictions as described in equation \ref{eq:reward}.

During the training of our privileged Scene Exploration Agent, we start every episode form a scene generated by the Scene Generation Agent. At every step the privileged Scene Exploration Agent takes as input the complete scene graph, and decides which object should be picked and where it should be placed. At every step the image of the scene is passed through an object detector to detect objects visible to the agent. 
If a new object is discovered, the agent receives a positive reward. If the agent makes a move that destabilizes the scene we terminate the episode and give the agent a negative reward (similar to the Scene Generation Agent training setup).
For both scene generation and scene exploration environments we use a disembodied agent that can move objects from one location to another, abstracting away trajectory planning and execution. 

A robotic manipulator can be added during test time with ease, as demonstrated in our video, to execute the learned policies. 
Further, to ensure that the scene is stable, we impart a small velocity of magnitude $7$cm/s along a randomly sampled unit vector on the XY plane, to the picked up object after placing it at it's destination. 
This mimics real world manipulation error and ensures that if the object is at equilibrium, it is at a \emph{stable} equilibrium. This ensures that the agent's intuition about physical plausibility learned in simulation can be reliably transferred to the real world. We also add constraints that limit the number of objects the agent can place on the tray. This ensures that instead of just trying to move all occluding objects onto the tray, the agent has to actively reason about rearranging the scene configuration to reveal hiding objects efficiently.

Our framework involves an inference step from the the CNN based object detector to compute the reward, which can be a bottleneck while training our agents. We tackle this problem by taking a multi-threaded approach. 
We create multiple processes each running simulations in parallel over multiple GPUs. 
We gather the rendered images from these processes at every step, batch them together, and run them though our object detector to get the predictions in a single pass. 
In our experiments, we simulated $35$ environments in parallel over $8$ GPUs, synchronously stepping through the environment while sharing a single copy of the object detection and policy neural networks.

\newpage
\added{
\begin{figure*}[h]
\centering
\includegraphics[width=0.98\linewidth]{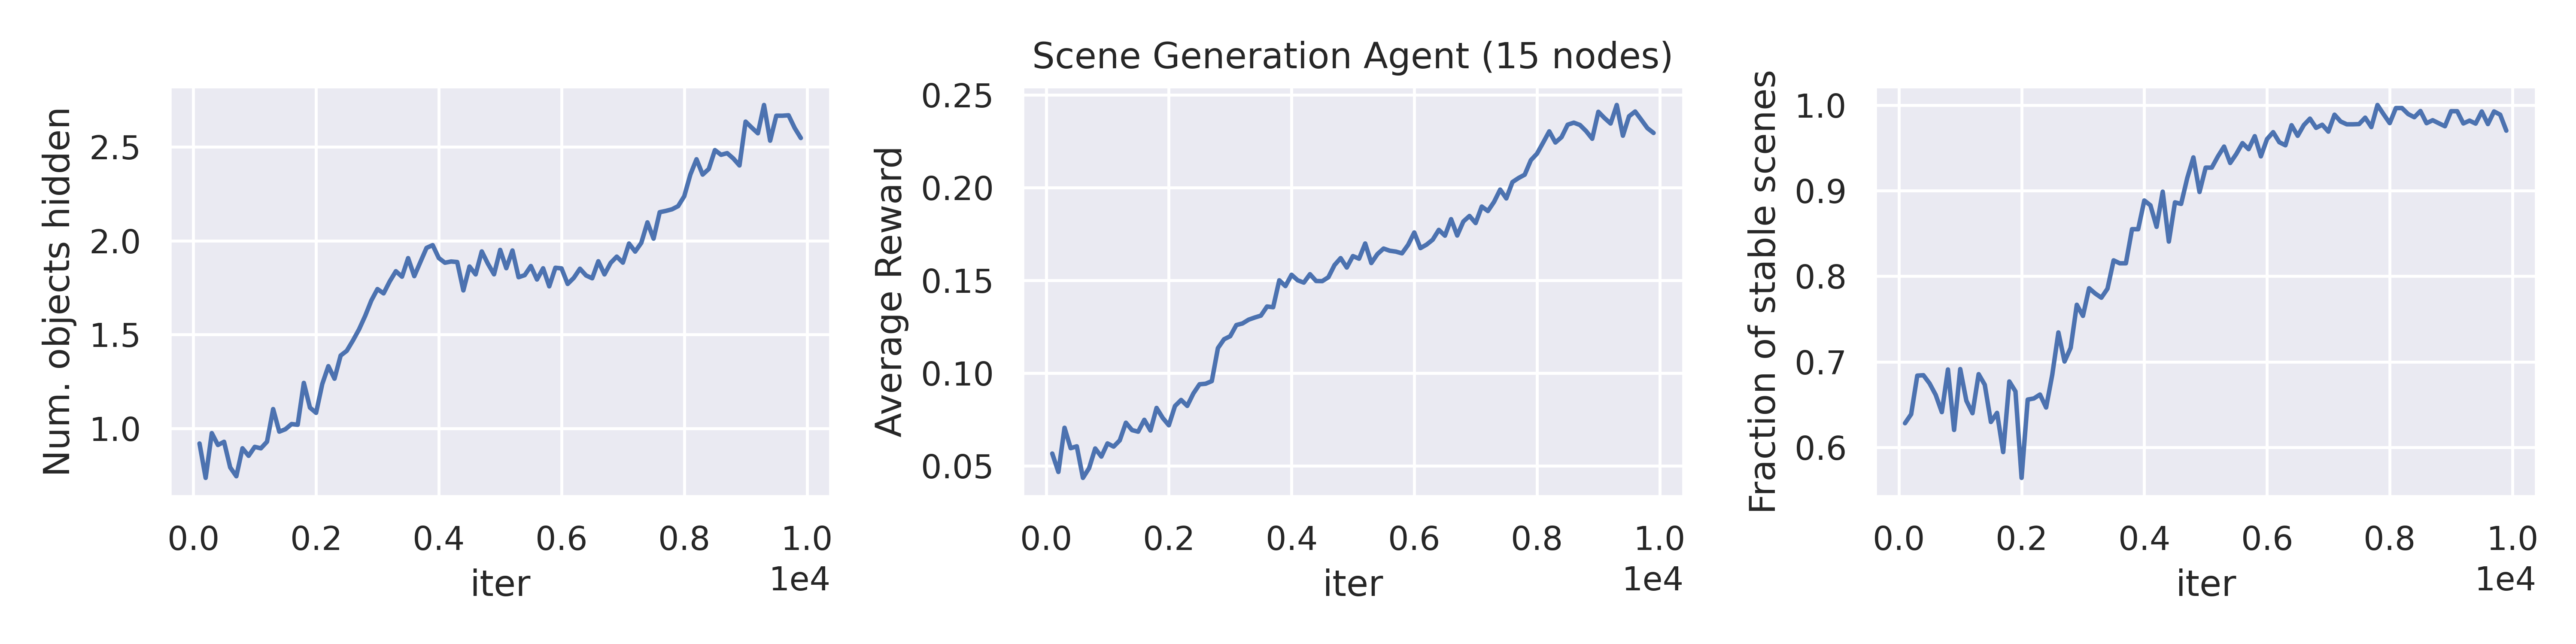}
\label{fig:training_scene_generation_15_nodes}
\caption{Training curves for scene generation agent with 15 graph nodes.}
% \sehoon{This is good. Can you add captions to the graph (with circles). People will not know it without reading figures.}}
\end{figure*}
\begin{figure*}[h]
\centering
\includegraphics[width=0.98\linewidth]{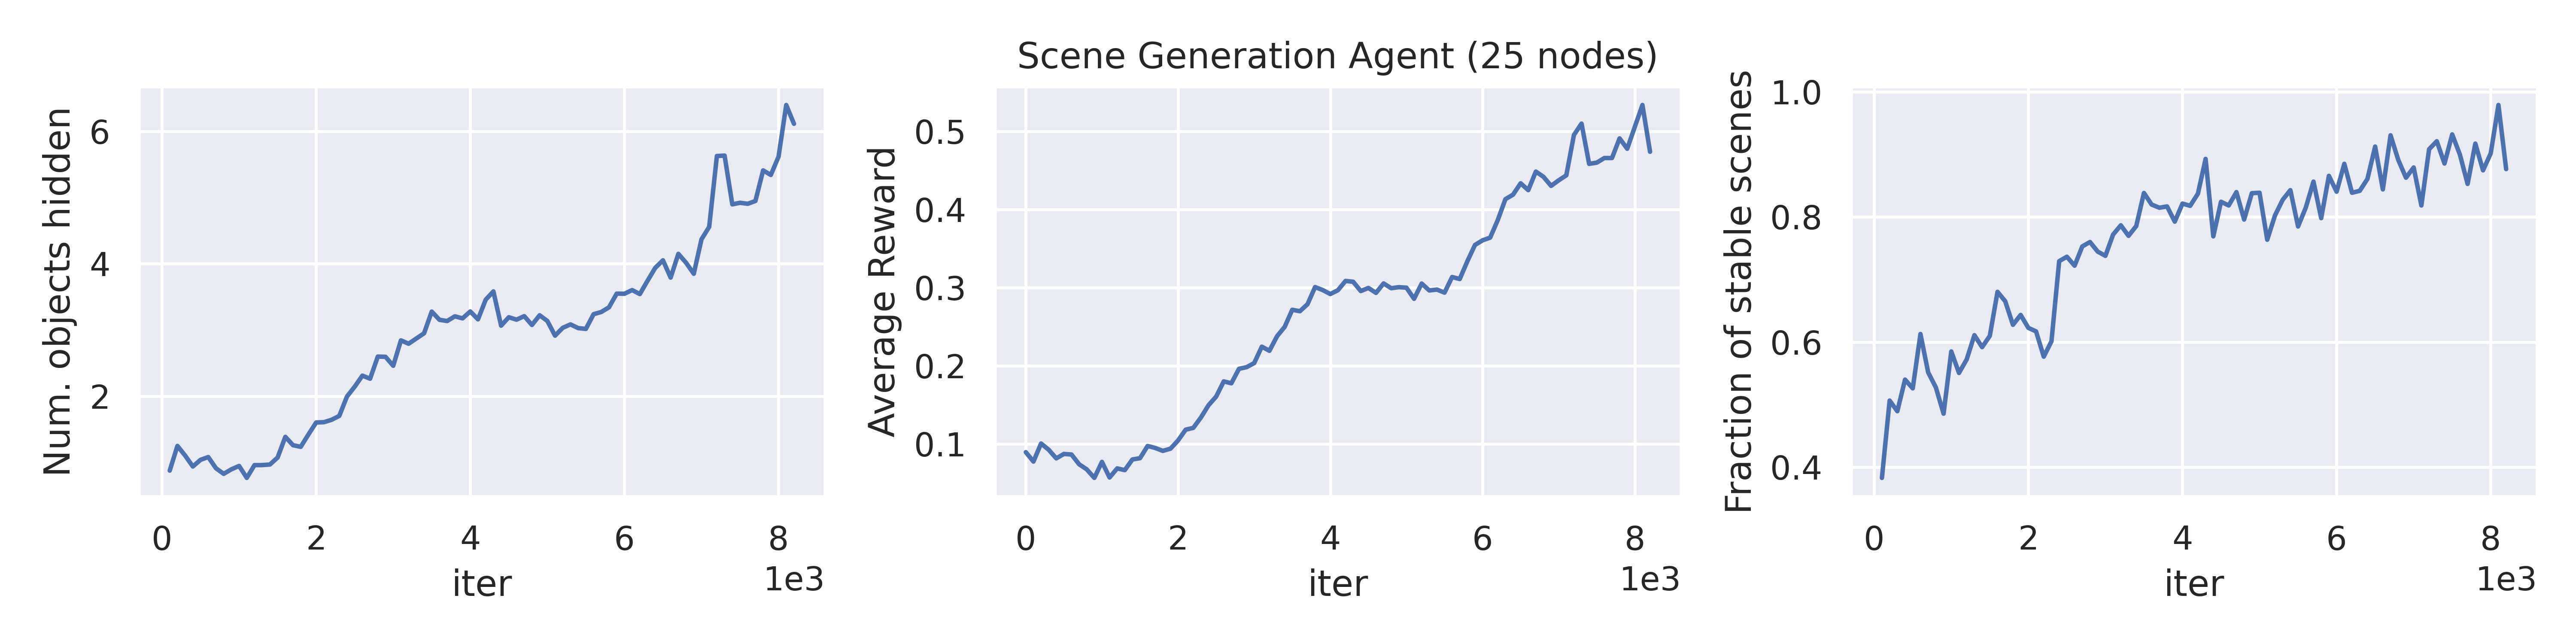}
\label{fig:training_scene_generation_25_nodes}
\caption{Training curves for scene generation agent with 25 graph nodes.}
% \sehoon{This is good. Can you add captions to the graph (with circles). People will not know it without reading figures.}}
\end{figure*}
\begin{figure*}[h]
\centering
\includegraphics[width=0.98\linewidth]{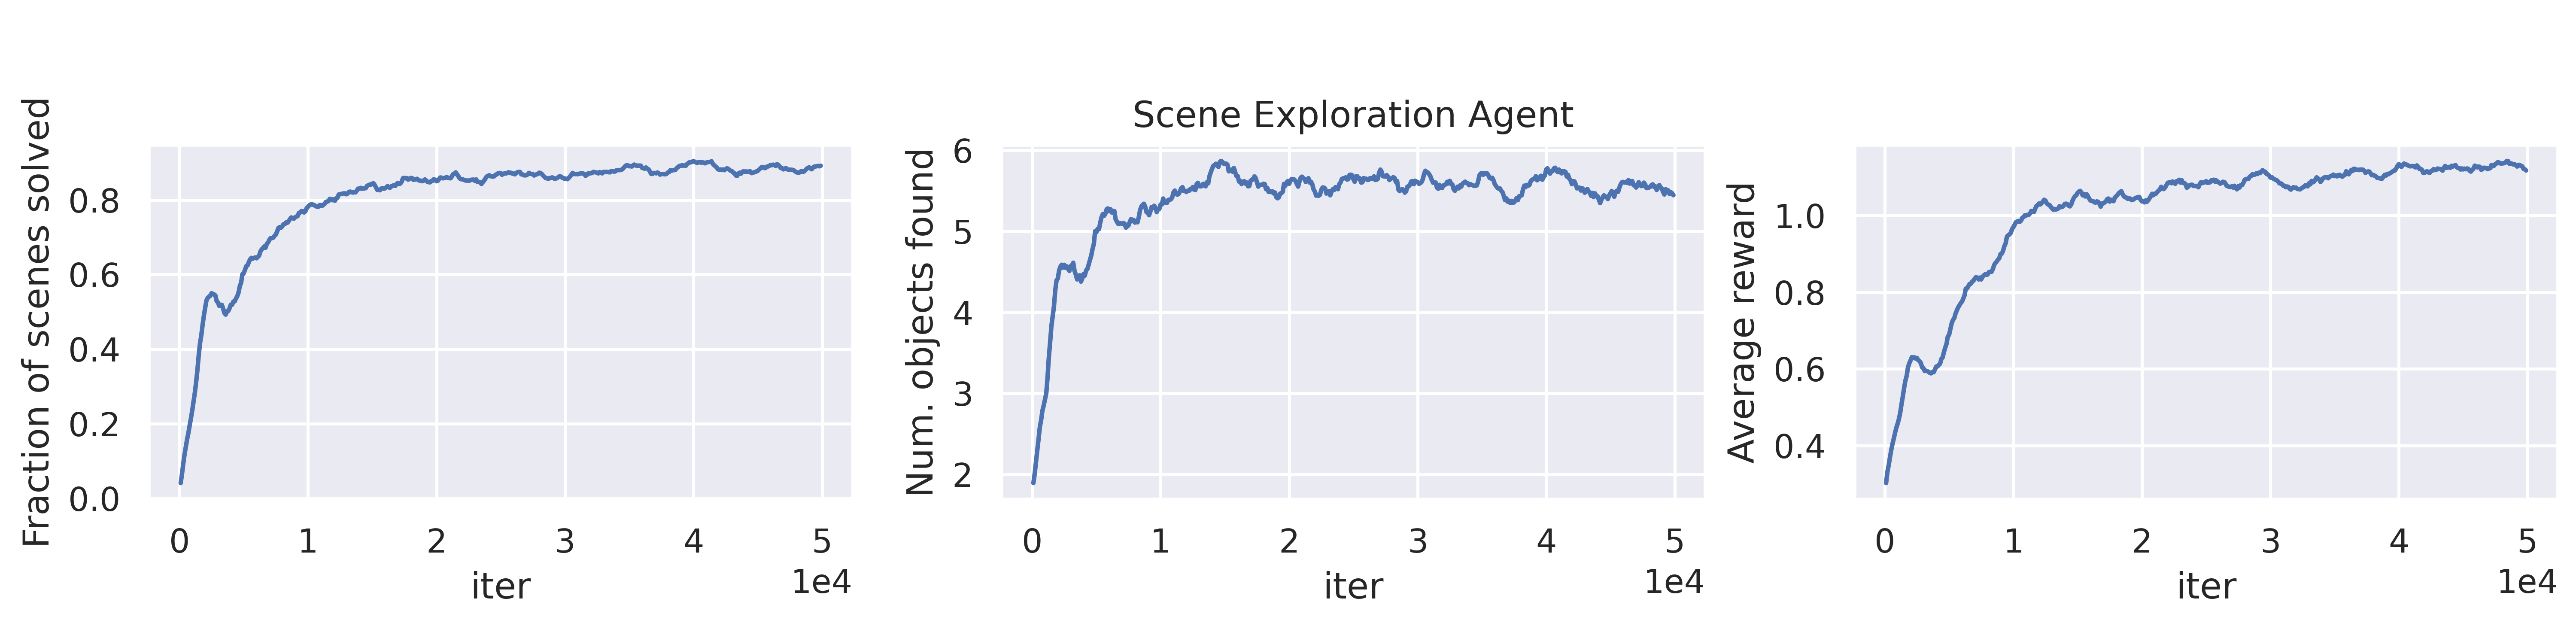}
\label{fig:training_scene_exploration}
\caption{Training curves for Privileged Scene Exploration Agent with 25 graph nodes.}
% \sehoon{This is good. Can you add captions to the graph (with circles). People will not know it without reading figures.}}
\end{figure*}
}
